# Supplementary material for: An Interpretable Rule Creation Method for Black-Box Models based on Surrogate Trees -- SRules
Source: arXiv:2407.20070 source file (2024-07-29)
Supplement: Supplementary file 1 [file Old_appendix.tex]

\appendix
\section{Annexes}


\subsection{Results}

\begin{table}
 \centering
 \caption{Selected Hiperparameters for SRules}

\resizebox{\columnwidth}{!}{%

\begin{tabular}{lll|cccc}
 \hline
\textbf{Dataset} & \textbf{Method} & \textbf{Recursive} & \textbf{p-significance} & \textbf{$\alpha$} & \textbf{minImp} & \textbf{minInsNode} \\ \hline
divorce & CAT & False & 0.95 & 0.95 & 0.05 & 5 \\
divorce & CAT & True & 0.95 & 0.95 & 0.05 & 5 \\
divorce & ADA & False & 0.95 & 0.95 & 0.05 & 5 \\
divorce & ADA & True & 0.95 & 0.95 & 0.05 & 5 \\
divorce & GBC & False & 0.95 & 0.95 & 0.05 & 5 \\
divorce & GBC & True & 0.95 & 0.95 & 0.05 & 5 \\
divorce & RF & False & 0.95 & 0.95 & 0.05 & 5 \\
divorce & RF & True & 0.95 & 0.95 & 0.05 & 5 \\ \hline
kr-vs-kp & CAT & False & 0.95 & 0.95 & 0.05 & 50 \\
kr-vs-kp & CAT & True & 0.95 & 0.95 & 0.05 & 5 \\
kr-vs-kp & ADA & False & 0.95 & 0.95 & 0.05 & 5 \\
kr-vs-kp & ADA & True & 0.95 & 0.95 & 0.05 & 5 \\
kr-vs-kp & GBC & False & 0.95 & 0.95 & 0.05 & 25 \\
kr-vs-kp & GBC & True & 0.95 & 0.95 & 0.05 & 10 \\
kr-vs-kp & RF & False & 0.95 & 0.95 & 0.05 & 10 \\
kr-vs-kp & RF & True & 0.95 & 0.95 & 0.05 & 5 \\ \hline
salud-covid & CAT & False & 0.95 & 0.95 & 0.05 & 5 \\
salud-covid & CAT & True & 0.95 & 0.95 & 0.05 & 5 \\
salud-covid & ADA & False & 0.95 & 0.95 & 0.05 & 5 \\
salud-covid & ADA & True & 0.95 & 0.95 & 0.05 & 5 \\
salud-covid & GBC & False & 0.95 & 0.95 & 0.05 & 5 \\
salud-covid & GBC & True & 0.95 & 0.95 & 0.05 & 5 \\
salud-covid & RF & False & 0.95 & 0.95 & 0.05 & 5 \\
salud-covid & RF & True & 0.95 & 0.95 & 0.05 & 5 \\ \hline
SPECT & CAT & False & 0.95 & 0.95 & 0.05 & 5 \\
SPECT & CAT & True & 0.95 & 0.95 & 0.05 & 10 \\
SPECT & ADA & False & 0.95 & 0.95 & 0.05 & 50 \\
SPECT & ADA & True & 0.95 & 0.95 & 0.05 & 5 \\
SPECT & GBC & False & 0.95 & 0.95 & 0.05 & 25 \\
SPECT & GBC & True & 0.95 & 0.95 & 0.05 & 50 \\
SPECT & RF & False & 0.95 & 0.95 & 0.05 & 50 \\
SPECT & RF & True & 0.95 & 0.95 & 0.05 & 50 \\ \hline
tic-tac-toe & CAT & False & 0.95 & 0.95 & 0.05 & 5 \\
tic-tac-toe & CAT & True & 0.95 & 0.95 & 0.05 & 5 \\
tic-tac-toe & ADA & False & 0.95 & 0.95 & 0.05 & 5 \\
tic-tac-toe & ADA & True & 0.95 & 0.95 & 0.05 & 5 \\
tic-tac-toe & GBC & False & 0.95 & 0.95 & 0.05 & 5 \\
tic-tac-toe & GBC & True & 0.95 & 0.95 & 0.05 & 5 \\
tic-tac-toe & RF & False & 0.95 & 0.95 & 0.05 & 5 \\
tic-tac-toe & RF & True & 0.95 & 0.95 & 0.05 & 5 \\ \hline
wisconsin & CAT & False & 0.95 & 0.95 & 0.05 & 5 \\
wisconsin & CAT & True & 0.95 & 0.95 & 0.05 & 5 \\
wisconsin & ADA & False & 0.95 & 0.95 & 0.05 & 5 \\
wisconsin & ADA & True & 0.95 & 0.95 & 0.05 & 5 \\
wisconsin & GBC & False & 0.95 & 0.95 & 0.05 & 5 \\
wisconsin & GBC & True & 0.95 & 0.95 & 0.05 & 5 \\
wisconsin & RF & False & 0.95 & 0.95 & 0.05 & 5 \\
wisconsin & RF & True & 0.95 & 0.95 & 0.05 & 5 \\ \hline
\end{tabular}
 } 
 \label{table:hyperparameters}
\end{table}


\begin{table}
 \centering
 \caption{Ensemble Non Recursive F1-score}

\resizebox{\columnwidth}{!}{%
 \begin{tabular}{c||c||c||c|c|cc|cc|cc}
 \hline
\textbf{Method}& \textbf{Dataset}  & \textbf{Coverage} & \textbf{DT} & \textbf{Ensemble} & \textbf{RFIT} & \textbf{RFIT \# rl. num.} & \textbf{RC} & \textbf{RC \# rl. num.} & \textbf{SR} & \textbf{SR \# rl. num.} \\ \hline 
 RF & divorce & 90.78±14.22 & 87.4±29.47 & 88.55±29.63 & 87.9±29.49 & 25.73±3.64 & 87.55±29.53 & 5.63±0.55 & 86.5±29.37 & 2.83±0.69 \\ 
 RF & kr-vs-kp & 75.12±5.54 & 98.04±1.5 & 99.84±0.22 & 98.86±0.97 & 21.9±2.86 & 94.25±1.62 & 4.1±0.3 & 98.91±1.03 & 10.8±1.356 \\ 
 RF & wisconsin & 71.04±12.58 & 98.44±1.73 & 98.83±1.28 & 99.03±1.51 & 19.1±2.13 & 98.69±1.49 & 8.47±1.38 & 98.49±1.77 & 5.03±1.82 \\ 
 RF & SPECT & 40.37±5.78 & 93.5±3.19 & 93.5±3.19 & 94.76±4.31 & 22.88±1.69 & 93.5±3.19 & 5.0±1.0 & 93.5±3.19 & 1.0±0.0 \\
 RF & salud-covid & 52.88±9.68 & 70.19±13.28 & 76.73±9.72 & 71.55±15.56 & 18.93±1.75 & 58.07±24.15 & 6.43±1.26 & 77.88±9.98 & 11.6±2.27\\
 RF & tic-tac-toe & 45.31±8.14 & 97.04±3.48 & 99.73±0.6 & 97.92±3.11 & 21.03±1.87 & 87.8±4.93 & 3.6±0.55 & 98.93±1.4 & 22.67±3.75\\ \hline
 RF & Total Average & 62.58±9.32 &	90.77±8.78 &	92.86±7.44 &	91.67±9.16 &	21.60±2.32 &	86.64±10.82 &	5.54±0.84 &	92.37±7.79 &	8.99±1.65\\ \hline


 GBC & divorce & 90.78±14.22 & 87.4±29.47 & 88.55±29.63 & 87.9±29.49 & 25.73±3.64 & 87.55±29.53 & 5.63±0.55 & 86.5±29.37 & 2.83±0.69 \\ 
 GBC & kr-vs-kp & 75.83±5.75 & 98.0±1.64 & 99.77±0.28 & 98.91±0.9 & 21.8±3.21 & 94.33±1.58 & 4.23±0.42 & 98.96±0.81 & 11.03±1.43 \\ 
 GBC & wisconsin & 71.04±12.58 & 98.44±1.73 & 98.83±1.28 & 99.03±1.51 & 19.1±2.13 & 98.69±1.49 & 8.47±1.38 & 98.49±1.77 & 5.03±1.82 \\ 
 GBC & SPECT & 42.57±14.73 & 93.41±5.29 & 94.82±3.88 & 95.59±3.99 & 21.67±2.87 & 94.82±3.88 & 4.75±0.6 & 94.82±3.88 & 1.25±0.43 \\
 GBC & salud-covid & 52.88±9.68 & 70.19±13.28 & 76.73±9.72 & 71.55±15.56 & 18.93±1.75 & 58.07±24.15 & 6.43±1.26 & 77.88±9.98 & 11.6±2.27 \\
 GBC & tic-tac-toe & 45.31±8.14 & 97.04±3.48 & 99.73±0.6 & 97.92±3.11 & 21.03±1.87 & 87.8±4.93 & 3.6±0.55 & 98.93±1.4 & 22.67±3.75\\\hline
 GBC & Total Average & 63.07±10.85	&90.75±9.15	&93.07±7.57	&91.82±9.09&	21.38±2.58	&86.88±10.93	&5.52±0.79	&92.60±7.87&	9.07±1.73\\ \hline

 ADA & divorce & 94.31±6.35 & 96.84±4.56 & 97.48±4.11 & 98.13±3.21 & 25.77±4.1 & 96.3±5.18 & 5.7±0.59 & 96.92±4.41 & 3.07±0.685 \\ 
 ADA & kr-vs-kp & 57.91±12.51 & 94.82±2.09 & 97.78±0.89 & 97.31±1.68 & 21.97±3.03 & 90.77±2.64 & 4.17±0.37 & 98.63±0.85 & 69.4±10.14 \\ 
 ADA & wisconsin & 75.38±10.07 & 98.02±1.41 & 98.74±1.14 & 98.83±1.09 & 18.83±2.16 & 98.38±1.33 & 8.3±1.51 & 97.74±1.15 & 8.47±2.11 \\ 
 ADA & SPECT & 29.63±0.0 & 85.71±0.0 & 85.71±0.0 & 85.71±0.0 & 22.0±0.0 & 85.71±0.0 & 6.0±0.0 & 85.71±0.0 & 1.0±0.0 \\
 ADA & salud-covid & 38.77±8.26 & 39.66±31.56 & 40.83±34.75 & 36.55±34.05 & 18.67±1.78 & 28.97±33.52 & 6.47±0.96 & 23.73±33.76 & 10.2±2.95 \\
 ADA & tic-tac-toe & 53.16±8.58 & 95.3±5.42 & 99.54±0.89 & 97.39±2.77 & 22.0±2.24 & 86.43±5.14 & 3.67±0.6 & 98.87±1.53 & 20.37±2.54 \\ \hline 
 ADA & Total Average & 58.19±7.63 & 85.06±7.51 & 86.68±6.96 & 85.65±7.13 & 21.54±2.22 & 81.09±7.97 & 5.72±0.67 & 83.60±6.95 & 18.75±3.07\\ \hline


 CAT & divorce & 92.16±11.7 & 94.16±18.0 & 63.38±12.39 & 95.13±17.96 & 24.17±3.26 & 93.96±17.96 & 5.7±0.59 & 95.06±17.91 & 3.07±0.63 \\ 
 CAT & kr-vs-kp & 49.95±9.56 & 99.28±1.66 & 59.54±6.8 & 99.27±1.66 & 21.23±3.57 & 91.3±4.12 & 4.07±0.25 & 99.28±1.66 & 3.2±0.65 \\ 
 CAT & wisconsin & 84.96±4.34 & 98.34±1.09 & 82.36±2.26 & 99.1±0.94 & 19.57±3.06 & 98.39±1.61 & 8.27±1.65 & 98.98±0.85 & 8.6±1.45 \\ 
 CAT & SPECT & 39.96±14.42 & 95.31±4.52 & 95.9±3.97 & 96.0±3.86 & 21.72±2.33 & 95.51±3.83 & 5.38±0.96 & 95.9±3.97 & 2.97±1.1 \\
 CAT & salud-covid & 43.88±9.94 & 74.74±19.07 & 14.33±4.66 & 86.53±14.54 & 18.33±1.89 & 76.81±22.13 & 6.17±0.73 & 87.76±12.66 & 7.4±1.84 \\
 CAT & tic-tac-toe & 49.03±6.29 & 99.48±0.88 & 88.16±3.02 & 100.0±0.0 & 21.33±1.64 & 95.79±4.46 & 3.53±0.56 & 99.66±0.85 & 11.17±2.6 \\ \hline
 CAT & Total Average & 59.99±9.375& 93.55±7.53& 67.27±5.51 & 96.00±6.49 & 21.05±2.625 & 91.96±9.02 & 5.52±0.79 & 96.10±6.31 & 5.20±1.18\\ \hline \hline

 
    \textbf{Global} & \textbf{Total Average} & \textbf{60.96±9.29} & \textbf{90.03±8.24} & \textbf{84.97±6.87} & \textbf{91.29±7.97} & \textbf{21.39±2.44} & \textbf{86.64±9.69} & \textbf{5.58±0.77} & \textbf{91.17±7.23} & \textbf{10.50±1.85} \\ \hline \hline
 \end{tabular}
 } 
 \label{table:results_table_non_recursive}
\end{table}

\begin{table}
 \centering
 \caption{Ensemble Recursive F1-score}

\resizebox{\columnwidth}{!}{%
 \begin{tabular}{c||c||c||c|c|cc|cc|cc}
 \hline

\textbf{Method}& \textbf{Dataset}  & \textbf{Coverage} & \textbf{DT} & \textbf{Ensemble} & \textbf{RFIT} & \textbf{RFIT \# rl. num.} & \textbf{RC} & \textbf{RC \# rl. num.} & \textbf{SR} & \textbf{SR \# rl. num.} \\ \hline
 RF & divorce & 91.96±14.68 & 88.94±24.74 & 51.56±44.22 & 88.54±29.63 & 26.47±3.95 & 87.1±29.33 & 5.67±0.54 & 86.17±29.19 & 3.0±1.34 \\ 
 RF & kr-vs-kp & 92.07±6.47 & 96.19±1.36 & 45.32±20.09 & 97.89±1.27 & 21.57±2.53 & 92.42±1.91 & 4.13±0.34 & 98.5±1.48 & 20.3±3.94 \\ 
 RF & wisconsin & 81.79±11.25 & 97.12±2.01 & 86.72±17.84 & 98.26±1.48 & 19.13±2.9 & 97.85±1.62 & 8.43±2.14 & 97.34±2.03 & 7.33±2.01 \\ 
 RF & SPECT & 50.62±5.52 & 89.83±2.12 & 89.15±9.57 & 89.83±2.12 & 21.5±2.5 & 89.83±2.12 & 5.67±1.7 & 90.62±3.06 & 1.0±0.0 \\
 RF & salud-covid & 60.13±5.56 & 64.2±19.59 & 40.54±15.13 & 69.35±16.39 & 18.5±1.89 & 56.22±19.84 & 6.07±1.18 & 74.54±13.28 & 15.3±3.08\\
 RF & tic-tac-toe & 68.65±10.02 & 95.91±3.83 & 76.16±10.5 & 97.38±2.21 & 21.13±2.01 & 85.94±4.49 & 3.6±0.49 & 98.35±1.93 & 33.23±5.55\\ \hline
 RF & Total Average & 74.20±8.92 & 88.70±8.94 & 64.91±19.56 & 90.21±8.85 & 21.38±2.63 & 84.89±9.89 & 5.60±1.07 & 90.92±8.50 & 13.36±2.65\\ \hline 


 GBC & divorce & 91.96±14.68 & 88.94±24.74 & 51.56±44.22 & 88.54±29.63 & 26.47±3.95 & 87.1±29.33 & 5.67±0.54 & 86.17±29.19 & 3.0±1.34 \\ 
 GBC & kr-vs-kp & 93.5±4.7 & 95.87±1.36 & 52.46±17.44 & 98.0±1.16 & 22.53±3.83 & 91.91±1.94 & 4.07±0.25 & 98.6±1.08 & 18.33±2.66 \\ 
 GBC & wisconsin & 81.79±11.25 & 97.12±2.01 & 86.72±17.84 & 98.26±1.48 & 19.13±2.9 & 97.85±1.62 & 8.43±2.14 & 97.34±2.03 & 7.33±2.01 \\ 
 GBC & SPECT & 50.62±5.52 & 89.83±2.12 & 89.15±9.57 & 89.83±2.12 & 21.5±2.5 & 89.83±2.12 & 5.67±1.7 & 90.62±3.06 & 1.0±0.0 \\
 GBC & salud-covid & 60.13±5.56 & 64.2±19.59 & 40.54±15.13 & 69.35±16.39 & 18.5±1.89 & 56.22±19.84 & 6.07±1.18 & 74.54±13.28 & 15.3±3.08\\
 GBC & tic-tac-toe & 68.65±10.02 & 95.91±3.83 & 76.16±10.5 & 97.38±2.21 & 21.13±2.01 & 85.94±4.49 & 3.6±0.49 & 98.35±1.93 & 33.23±5.55\\ \hline
 GBC & Total Average & 74.44±8.62 &	88.65±8.94 &	66.10±19.12 &	90.23±8.83 &	21.54±2.85 &	84.81±9.89 &	5.59±1.05 &	90.94±8.43 &	13.03±2.44\\ \hline



 ADA &	divorce & 93.14±9.74 & 92.61±17.75 & 65.76±38.3 & 94.45±17.83 & 24.97±2.27 & 92.48±17.79 & 5.7±0.59 & 91.89±17.82 & 3.8±1.8 \\ 
 ADA &	kr-vs-kp & 83.45±5.82 & 95.53±1.06 & 80.55±12.44 & 97.33±1.26 & 21.73±3.13 & 91.92±1.86 & 4.1±0.3 & 95.85±3.44 & 106.3±14.45 \\ 
 ADA &	wisconsin & 81.24±7.57 & 97.57±2.11 & 87.99±14.52 & 98.61±1.15 & 19.37±2.21 & 98.3±1.38 & 8.63±1.91 & 97.13±2.29 & 8.83±2.1 \\ 
 ADA &	SPECT & 28.28±14.42 & 92.38±8.13 & 88.83±19.55 & 91.19±18.48 & 22.18±1.93 & 93.91±6.69 & 5.29±1.1 & 94.1±6.93 & 3.61±1.29 \\
 ADA &	salud-covid & 52.28±7.1 & 52.32±22.95 & 46.69±19.69 & 53.33±23.21 & 18.03±1.64 & 33.77±25.26 & 6.27±1.0 & 43.2±31.03 & 21.33±7.03 \\
 ADA &	tic-tac-toe & 72.2±7.49 & 95.14±4.28 & 86.57±4.9 & 97.31±2.01 & 22.13±2.31 & 84.3±4.59 & 3.7±0.74 & 99.23±0.97 & 31.0±4.43 \\ \hline
 ADA &	Total Average & 68.43±8.69 &	87.59±9.38 &	76.07±18.23 &	88.70±10.66 &	21.40±2.25 &	82.45±9.60 &	5.62±0.94 &	86.90±10.41 &	29.15±5.18\\ \hline


 CAT & divorce & 93.92±6.35 & 98.49±2.76 & 65.75±3.49 & 98.66±3.14 & 25.5±3.37 & 97.03±4.86 & 5.73±0.57 & 98.06±2.98 & 3.73±1.77 \\ 
 CAT & kr-vs-kp & 89.99±4.03 & 96.88±1.83 & 69.76±2.66 & 98.43±1.08 & 21.47±3.06 & 93.05±2.42 & 4.13±0.34 & 98.76±1.11 & 16.23±3.5 \\ 
 CAT & wisconsin & 87.07±5.25 & 98.04±1.63 & 81.77±2.25 & 99.17±1.2 & 18.93±1.77 & 98.38±1.72 & 8.0±1.53 & 98.64±1.52 & 9.2±1.17 \\ 
 CAT & SPECT & 45.0±15.13 & 94.69±5.37 & 95.81±4.68 & 95.99±4.74 & 21.85±2.63 & 95.68±4.71 & 5.44±1.37 & 95.81±4.68 & 2.7±1.41 \\
 CAT & salud-covid & 58.28±6.1 & 64.37±20.78 & 15.29±4.05 & 71.47±14.13 & 18.5±1.96 & 58.35±21.51 & 6.4±1.08 & 73.47±15.63 & 12.0±2.83\\
 CAT & tic-tac-toe & 62.77±6.25 & 97.54±1.66 & 84.68±3.42 & 98.26±1.76 & 21.4±1.85 & 91.38±4.3 & 3.8±0.54 & 98.64±1.26 & 21.43±4.35 \\ \hline 
 CAT & Total Average & 72.84±7.19 & 91.67±5.67 & 68.84±3.43 & 93.66±4.34 & 21.28±2.44 & 88.98±6.59 & 5.58±0.91 & 93.90±4.53 & 10.88±2.51\\ \hline \hline

     \textbf{Global}& \textbf{Total Average} & \textbf{72.48±8.36} & \textbf{89.15±8.23} & \textbf{68.98±15.09} & \textbf{90.70±8.17} & \textbf{21.40±2.54} & \textbf{85.28±8.99} & \textbf{5.60±0.99} & \textbf{90.67±7.97} & \textbf{16.61±3.15}\\ \hline \hline

 \end{tabular}
 } 
 \label{table:results_table_recursive}
\end{table}




%% divorce
\subsection{divorce}
\begin{figure}[H]
 \centering
 
 \begin{subfigure}[b]{0.225\textwidth}
 \centering
 \includegraphics[width=\textwidth]{images/battery_divorce_<catboost.core.CatBoostClassifier object at 0x7f799c1b7fd0>_False.png}
 \caption{CAT - NR}
 \label{fig:divorce_CAT_non_R}
 \end{subfigure}
 \hfill
 \begin{subfigure}[b]{0.225\textwidth}
 \centering
 \includegraphics[width=\textwidth]{images/battery_divorce_AdaBoostClassifier()_False.png}
 \caption{ADA - NR}
 \label{fig:divorce_ADA_non_R}
 \end{subfigure}
 \hfill
 \begin{subfigure}[b]{0.225\textwidth}
 \centering
 \includegraphics[width=\textwidth]{images/battery_divorce_GradientBoostingClassifier()_False.png}
 \caption{GBC - NR}
 \label{fig:divorce_GBC_non_R}
 \end{subfigure}
 \hfill
 \begin{subfigure}[b]{0.225\textwidth}
 \centering
 \includegraphics[width=\textwidth]{images/battery_divorce_RandomForestClassifier()_False.png}
 \caption{RF - NR}
 \label{fig:divorce_RF_non_R}
 \end{subfigure}
 \hfill

%% BELLOW
 \centering
 \begin{subfigure}[b]{0.225\textwidth}
 \centering
 \includegraphics[width=\textwidth]{images/battery_divorce_<catboost.core.CatBoostClassifier object at 0x7f799c1b7fd0>_True.png}
 \caption{CAT - R}
 \label{fig:divorce_CAT_R}
 \end{subfigure}
 \hfill
 \begin{subfigure}[b]{0.225\textwidth}
 \centering
 \includegraphics[width=\textwidth]{images/battery_divorce_AdaBoostClassifier()_True.png}
 \caption{ADA - R}
 \label{fig:divorce_ADA_R}
 \end{subfigure}
 \hfill
 \begin{subfigure}[b]{0.225\textwidth}
 \centering
 \includegraphics[width=\textwidth]{images/battery_divorce_GradientBoostingClassifier()_True.png}
 \caption{GBC - R}
 \label{fig:divorce_GBC_R}
 \end{subfigure}
 \hfill
 \begin{subfigure}[b]{0.225\textwidth}
 \centering
 \includegraphics[width=\textwidth]{images/battery_divorce_RandomForestClassifier()_True.png}
 \caption{RF - R}
 \label{fig:divorce_RF_R}
 \end{subfigure}
 \caption{divorce - comparison (NR: No Recursive, R: Recursive)}
 \label{fig:divorce:comparison}
\end{figure}


%% kr-vs-kp}
\subsection{kr-vs-kp}
\begin{figure}[H]
 \centering
 
 \begin{subfigure}[b]{0.225\textwidth}
 \centering
 \includegraphics[width=\textwidth]{images/battery_kr-vs-kp_<catboost.core.CatBoostClassifier object at 0x7f799c1b7fd0>_False.png}
 \caption{CAT - NR}
 \label{fig:kr-vs-kp_CAT_non_R}
 \end{subfigure}
 \hfill
 \begin{subfigure}[b]{0.225\textwidth}
 \centering
 \includegraphics[width=\textwidth]{images/battery_kr-vs-kp_AdaBoostClassifier()_False.png}
 \caption{ADA - NR}
 \label{fig:kr-vs-kp_ADA_non_R}
 \end{subfigure}
 \hfill
 \begin{subfigure}[b]{0.225\textwidth}
 \centering
 \includegraphics[width=\textwidth]{images/battery_kr-vs-kp_GradientBoostingClassifier()_False.png}
 \caption{GBC - NR}
 \label{fig:kr-vs-kp_GBC_non_R}
 \end{subfigure}
 \hfill
 \begin{subfigure}[b]{0.225\textwidth}
 \centering
 \includegraphics[width=\textwidth]{images/battery_kr-vs-kp_RandomForestClassifier()_False.png}
 \caption{RF - NR}
 \label{fig:kr-vs-kp_RF_non_R}
 \end{subfigure}
 \hfill

%% BELLOW
 \centering
 \begin{subfigure}[b]{0.225\textwidth}
 \centering
 \includegraphics[width=\textwidth]{images/battery_kr-vs-kp_<catboost.core.CatBoostClassifier object at 0x7f799c1b7fd0>_True.png}
 \caption{CAT - R}
 \label{fig:kr-vs-kp_CAT_R}
 \end{subfigure}
 \hfill
 \begin{subfigure}[b]{0.225\textwidth}
 \centering
 \includegraphics[width=\textwidth]{images/battery_kr-vs-kp_AdaBoostClassifier()_True.png}
 \caption{ADA - R}
 \label{fig:kr-vs-kp_ADA_R}
 \end{subfigure}
 \hfill
 \begin{subfigure}[b]{0.225\textwidth}
 \centering
 \includegraphics[width=\textwidth]{images/battery_kr-vs-kp_GradientBoostingClassifier()_True.png}
 \caption{GBC - R}
 \label{fig:kr-vs-kp_GBC_R}
 \end{subfigure}
 \hfill
 \begin{subfigure}[b]{0.225\textwidth}
 \centering
 \includegraphics[width=\textwidth]{images/battery_kr-vs-kp_RandomForestClassifier()_True.png}
 \caption{RF - R}
 \label{fig:kr-vs-kp_RF_R}
 \end{subfigure}
 \caption{kr-vs-kp - comparison (NR: No Recursive, R: Recursive)}
 \label{fig:kr-vs-kp:comparison}
\end{figure}


%% wisconsin}
\subsection{wisconsin}
\begin{figure}[H]
 \centering
 
 \begin{subfigure}[b]{0.225\textwidth}
 \centering
 \includegraphics[width=\textwidth]{images/battery_wisconsin_<catboost.core.CatBoostClassifier object at 0x7f799c1b7fd0>_False.png}
 \caption{CAT - NR}
 \label{fig:wisconsin_CAT_non_R}
 \end{subfigure}
 \hfill
 \begin{subfigure}[b]{0.225\textwidth}
 \centering
 \includegraphics[width=\textwidth]{images/battery_wisconsin_AdaBoostClassifier()_False.png}
 \caption{ADA - NR}
 \label{fig:wisconsin_ADA_non_R}
 \end{subfigure}
 \hfill
 \begin{subfigure}[b]{0.225\textwidth}
 \centering
 \includegraphics[width=\textwidth]{images/battery_wisconsin_GradientBoostingClassifier()_False.png}
 \caption{GBC - NR}
 \label{fig:wisconsin_GBC_non_R}
 \end{subfigure}
 \hfill
 \begin{subfigure}[b]{0.225\textwidth}
 \centering
 \includegraphics[width=\textwidth]{images/battery_wisconsin_RandomForestClassifier()_False.png}
 \caption{RF - NR}
 \label{fig:wisconsin_RF_non_R}
 \end{subfigure}
 \hfill

%% BELLOW
 \centering
 \begin{subfigure}[b]{0.225\textwidth}
 \centering
 \includegraphics[width=\textwidth]{images/battery_wisconsin_<catboost.core.CatBoostClassifier object at 0x7f799c1b7fd0>_True.png}
 \caption{CAT - R}
 \label{fig:wisconsin_CAT_R}
 \end{subfigure}
 \hfill
 \begin{subfigure}[b]{0.225\textwidth}
 \centering
 \includegraphics[width=\textwidth]{images/battery_wisconsin_AdaBoostClassifier()_True.png}
 \caption{ADA - R}
 \label{fig:wisconsin_ADA_R}
 \end{subfigure}
 \hfill
 \begin{subfigure}[b]{0.225\textwidth}
 \centering
 \includegraphics[width=\textwidth]{images/battery_wisconsin_GradientBoostingClassifier()_True.png}
 \caption{GBC - R}
 \label{fig:wisconsin_GBC_R}
 \end{subfigure}
 \hfill
 \begin{subfigure}[b]{0.225\textwidth}
 \centering
 \includegraphics[width=\textwidth]{images/battery_wisconsin_RandomForestClassifier()_True.png}
 \caption{RF - R}
 \label{fig:wisconsin_RF_R}
 \end{subfigure}
 \caption{wisconsin - comparison (NR: No Recursive, R: Recursive)}
 \label{fig:wisconsin:comparison}
\end{figure}


%% SPECT}
\subsection{SPECT}
\begin{figure}[H]
 \centering
 
 \begin{subfigure}[b]{0.225\textwidth}
 \centering
 \includegraphics[width=\textwidth]{images/battery_SPECT_<catboost.core.CatBoostClassifier object at 0x7f799c1b7fd0>_False.png}
 \caption{CAT - NR}
 \label{fig:SPECT_CAT_non_R}
 \end{subfigure}
 \hfill
 \begin{subfigure}[b]{0.225\textwidth}
 \centering
 \includegraphics[width=\textwidth]{images/battery_SPECT_AdaBoostClassifier()_False.png}
 \caption{ADA - NR}
 \label{fig:SPECT_ADA_non_R}
 \end{subfigure}
 \hfill
 \begin{subfigure}[b]{0.225\textwidth}
 \centering
 \includegraphics[width=\textwidth]{images/battery_SPECT_GradientBoostingClassifier()_False.png}
 \caption{GBC - NR}
 \label{fig:SPECT_GBC_non_R}
 \end{subfigure}
 \hfill
 \begin{subfigure}[b]{0.225\textwidth}
 \centering
 \includegraphics[width=\textwidth]{images/battery_SPECT_RandomForestClassifier()_False.png}
 \caption{RF - NR}
 \label{fig:SPECT_RF_non_R}
 \end{subfigure}
 \hfill

%% BELLOW
 \centering
 \begin{subfigure}[b]{0.225\textwidth}
 \centering
 \includegraphics[width=\textwidth]{images/battery_SPECT_<catboost.core.CatBoostClassifier object at 0x7f799c1b7fd0>_True.png}
 \caption{CAT - R}
 \label{fig:SPECT_CAT_R}
 \end{subfigure}
 \hfill
 \begin{subfigure}[b]{0.225\textwidth}
 \centering
 \includegraphics[width=\textwidth]{images/battery_SPECT_AdaBoostClassifier()_True.png}
 \caption{ADA - R}
 \label{fig:SPECT_ADA_R}
 \end{subfigure}
 \hfill
 \begin{subfigure}[b]{0.225\textwidth}
 \centering
 \includegraphics[width=\textwidth]{images/battery_SPECT_GradientBoostingClassifier()_True.png}
 \caption{GBC - R}
 \label{fig:SPECT_GBC_R}
 \end{subfigure}
 \hfill
 \begin{subfigure}[b]{0.225\textwidth}
 \centering
 \includegraphics[width=\textwidth]{images/battery_SPECT_RandomForestClassifier()_True.png}
 \caption{RF - R}
 \label{fig:SPECT_RF_R}
 \end{subfigure}
 \caption{SPECT - comparison (NR: No Recursive, R: Recursive)}
 \label{fig:SPECT:comparison}
\end{figure}


%% salud-covid}
\subsection{salud-covid}
\begin{figure}[H]
 \centering
 
 \begin{subfigure}[b]{0.225\textwidth}
 \centering
 \includegraphics[width=\textwidth]{images/battery_salud-covid_<catboost.core.CatBoostClassifier object at 0x7f799c1b7fd0>_False.png}
 \caption{CAT - NR}
 \label{fig:salud-covid_CAT_non_R}
 \end{subfigure}
 \hfill
 \begin{subfigure}[b]{0.225\textwidth}
 \centering
 \includegraphics[width=\textwidth]{images/battery_salud-covid_AdaBoostClassifier()_False.png}
 \caption{ADA - NR}
 \label{fig:salud-covid_ADA_non_R}
 \end{subfigure}
 \hfill
 \begin{subfigure}[b]{0.225\textwidth}
 \centering
 \includegraphics[width=\textwidth]{images/battery_salud-covid_GradientBoostingClassifier()_False.png}
 \caption{GBC - NR}
 \label{fig:salud-covid_GBC_non_R}
 \end{subfigure}
 \hfill
 \begin{subfigure}[b]{0.225\textwidth}
 \centering
 \includegraphics[width=\textwidth]{images/battery_salud-covid_RandomForestClassifier()_False.png}
 \caption{RF - NR}
 \label{fig:salud-covid_RF_non_R}
 \end{subfigure}
 \hfill

%% BELLOW
 \centering
 \begin{subfigure}[b]{0.225\textwidth}
 \centering
 \includegraphics[width=\textwidth]{images/battery_salud-covid_<catboost.core.CatBoostClassifier object at 0x7f799c1b7fd0>_True.png}
 \caption{CAT - R}
 \label{fig:salud-covid_CAT_R}
 \end{subfigure}
 \hfill
 \begin{subfigure}[b]{0.225\textwidth}
 \centering
 \includegraphics[width=\textwidth]{images/battery_salud-covid_AdaBoostClassifier()_True.png}
 \caption{ADA - R}
 \label{fig:salud-covid_ADA_R}
 \end{subfigure}
 \hfill
 \begin{subfigure}[b]{0.225\textwidth}
 \centering
 \includegraphics[width=\textwidth]{images/battery_salud-covid_GradientBoostingClassifier()_True.png}
 \caption{GBC - R}
 \label{fig:salud-covid_GBC_R}
 \end{subfigure}
 \hfill
 \begin{subfigure}[b]{0.225\textwidth}
 \centering
 \includegraphics[width=\textwidth]{images/battery_salud-covid_RandomForestClassifier()_True.png}
 \caption{RF - R}
 \label{fig:salud-covid_RF_R}
 \end{subfigure}
 \caption{salud-covid - comparison (NR: No Recursive, R: Recursive)}
 \label{fig:salud-covid:comparison}
\end{figure}


%% tic-tac-toe}
\subsection{tic-tac-toe}
\begin{figure}[H]
 \centering
 
 \begin{subfigure}[b]{0.225\textwidth}
 \centering
 \includegraphics[width=\textwidth]{images/battery_tic-tac-toe_<catboost.core.CatBoostClassifier object at 0x7f799c1b7fd0>_False.png}
 \caption{CAT - NR}
 \label{fig:tic-tac-toe_CAT_non_R}
 \end{subfigure}
 \hfill
 \begin{subfigure}[b]{0.225\textwidth}
 \centering
 \includegraphics[width=\textwidth]{images/battery_tic-tac-toe_AdaBoostClassifier()_False.png}
 \caption{ADA - NR}
 \label{fig:tic-tac-toe_ADA_non_R}
 \end{subfigure}
 \hfill
 \begin{subfigure}[b]{0.225\textwidth}
 \centering
 \includegraphics[width=\textwidth]{images/battery_tic-tac-toe_GradientBoostingClassifier()_False.png}
 \caption{GBC - NR}
 \label{fig:tic-tac-toe_GBC_non_R}
 \end{subfigure}
 \hfill
 \begin{subfigure}[b]{0.225\textwidth}
 \centering
 \includegraphics[width=\textwidth]{images/battery_tic-tac-toe_RandomForestClassifier()_False.png}
 \caption{RF - NR}
 \label{fig:tic-tac-toe_RF_non_R}
 \end{subfigure}
 \hfill

%% BELLOW
 \centering
 \begin{subfigure}[b]{0.225\textwidth}
 \centering
 \includegraphics[width=\textwidth]{images/battery_tic-tac-toe_<catboost.core.CatBoostClassifier object at 0x7f799c1b7fd0>_True.png}
 \caption{CAT - R}
 \label{fig:tic-tac-toe_CAT_R}
 \end{subfigure}
 \hfill
 \begin{subfigure}[b]{0.225\textwidth}
 \centering
 \includegraphics[width=\textwidth]{images/battery_tic-tac-toe_AdaBoostClassifier()_True.png}
 \caption{ADA - R}
 \label{fig:tic-tac-toe_ADA_R}
 \end{subfigure}
 \hfill
 \begin{subfigure}[b]{0.225\textwidth}
 \centering
 \includegraphics[width=\textwidth]{images/battery_tic-tac-toe_GradientBoostingClassifier()_True.png}
 \caption{GBC - R}
 \label{fig:tic-tac-toe_GBC_R}
 \end{subfigure}
 \hfill
 \begin{subfigure}[b]{0.225\textwidth}
 \centering
 \includegraphics[width=\textwidth]{images/battery_tic-tac-toe_RandomForestClassifier()_True.png}
 \caption{RF - R}
 \label{fig:tic-tac-toe_RF_R}
 \end{subfigure}
 \caption{tic-tac-toe - comparison (NR: No Recursive, R: Recursive)}
 \label{fig:tic-tac-toe:comparison}
\end{figure}




\begin{figure}[H]
     \centering
     
     \begin{subfigure}[b]{0.32\textwidth}
         \centering
         \includegraphics[width=\textwidth]{images/battery_divorce_RandomForestClassifier()_False.png}
         \caption{divorce - NR}
         \label{fig:RF_divorce_non_R}
     \end{subfigure}
     \hfill
     \begin{subfigure}[b]{0.32\textwidth}
         \centering
         \includegraphics[width=\textwidth]{images/battery_kr-vs-kp_RandomForestClassifier()_False.png}
         \caption{kr-vs-kp - NR}
         \label{fig:RF_kr-vs-kp_non_R}
     \end{subfigure}
     \hfill
     \begin{subfigure}[b]{0.32\textwidth}
         \centering
         \includegraphics[width=\textwidth]{images/battery_wisconsin_RandomForestClassifier()_False.png}
         \caption{wisconsin - NR}
         \label{fig:RF_wisconsin_non_R}
     \end{subfigure}
     \hfill

%% BELLOW
     \centering
     \begin{subfigure}[b]{0.32\textwidth}
         \centering
         \includegraphics[width=\textwidth]{images/battery_divorce_RandomForestClassifier()_True.png}
         \caption{divorce - R}
         \label{fig:RF_divorce_R}
     \end{subfigure}
     \hfill
     \begin{subfigure}[b]{0.32\textwidth}
         \centering
         \includegraphics[width=\textwidth]{images/battery_kr-vs-kp_RandomForestClassifier()_True.png}
         \caption{kr-vs-kp - R}
         \label{fig:RF_kr-vs-kp_R}
     \end{subfigure}
     \hfill
     \begin{subfigure}[b]{0.32\textwidth}
         \centering
         \includegraphics[width=\textwidth]{images/battery_wisconsin_RandomForestClassifier()_True.png}
         \caption{Wisconsin - R}
         \label{fig:RF_wisconsin_R}
     \end{subfigure}
     \hfill
    \caption{Random Forest - comparison (NR: No Recursive, R: Recursive)}
     \label{fig:RF1:comparison}
\end{figure}
